# Supplementary material for: Positional Identifiability from Pairwise Collision Data
Source: arXiv:2605.23073 source file (2026-08-22)
Supplement: Supplementary file 1 [file appendix.tex]

\subsection{Proof for Theorem~\ref{lem:generalk}}\label{pf:generalk}
Let $\Earc=\{\e{a_1}{b_1},\ldots,\e{a_k}{b_k}\}$ and rearrange the entries in $\{a_1,b_1,\ldots,a_k,b_k\}$ into $(c_1,\ldots,c_2k)$ so that $c_1<\ldots<c_2k$, i.e., the sequence is increasing. Similar to what we did in the proof of Proposition~\ref{prop:k3}, we construct $h$ using a two-step approach. In the first step, we group the nodes $\dc_{c_1},\ldots,\dc_{c_{2k}}$. In the second step, we find a set of values $r_1,\ldots,r_{L}$ that satisfies Equations~\eqref{eq:diri} and~\eqref{eq:decidingr}, and the constraints on \textcolor{red}{$d_i$,} $i\in[L],$ that is consistent with the grouping of $c_1,\ldots,c_{2k}$ (which is \eqref{eq:group6} in the proof of Proposition \ref{prop:k3}).

Here, the grouping step generalizes that in the proof of Proposition~\ref{prop:k3} as described in Algorithm~\ref{alg:grouping}.
\begin{algorithm}
  \caption{Grouping of nodes $\{c_1,\ldots,c_{2k}\}$\iffalse$(\boldsymbol{a},\boldsymbol{b},\boldsymbol{c})$\fi} 
  \label{alg:grouping}
  \begin{algorithmic}[1]
    \STATE \textbf{Input:} $\Earc$.
    \STATE \textbf{Initialization:} Order the nodes in $\{\dc_{a_1},\ldots,\dc_{a_k},\dc_{b_1},\ldots,\dc_{b_k}\}$ as $\{\dc_{c_1},\ldots,\dc_{c_{2k}}\}$ such that $c_1<\ldots<c_{2k}$. Let
    $E_{adj} = \{\{c_i,c_{i+1}\}:i\in\{1,\ldots,2k--1\}\}$ and $E_{group}=\emptyset$.  
    \STATE \textbf{Step 1:} Find the pair $\{c_{i^*},c_{i^*+1}\}\in E_{adj}$ such that $\dc_{c_{i^*}},\dc_{c_{i^*+1}})\notin \Earc$ and $(c_{i^*+1}-c_{i^*})$ is as small as possible, i.e. $i^*=\arg\min_{\{c_{i},c_{i+1}\}\in E_{adj},(\dc_{c_{i}},\dc_{c_{i+1}})\notin \Earc}(c_{i+1}-c_i)$.
    \STATE \textbf{Step 2:} For each $c_i$ such that $(\dc_{c_{i}},\dc_{c_{i^*}})\in \Earc$ or $(\dc_{c_{i}},\dc_{c_{i^*+1}})\in \Earc$, and each $c_j$ such that $(\dc_{c_j},\dc_{c_{i-1}})\in \Earc$ or $(\dc_{c_j},\dc_{c_{i+1}})\in \Earc$, remove $\{c_{j},c_{j+1}\}$ from $E_{adj}$ if $\{c_{j},c_{j+1}\}\in E_{adj}$. Remove $\{c_{i^*},c_{i^*+1}\}$ from $E_{adj}$ if $\{c_{i^*},c_{i^*+1}\}\in E_{adj}$. Add $\{c_{i^*},c_{i^*+1}\}$ to $E_{group}$, i.e., $E_{group}=E_{group}\cup \{\{c_{i^*},c_{i^*+1}\}\}$.  
    \STATE \textbf{Step 3:} If $E_{adj}\ne \emptyset$, go to \textbf{Step 1}. 
    \STATE \textbf{Return} $E_{group}\cup \{\{c_i\}\}_{\{c_i,c_{i+1}\}\notin E_{group}, \{c_{i-1},c_i\}\notin E_{group}}$.
  \end{algorithmic}
\end{algorithm}
We have the following proposition for the output $E_{group}$ of Algorithm \ref{alg:grouping}.
\begin{proposition}
The output $E_{group}$ of Algorithm~\ref{alg:grouping} satisfies $|E_{group}|\le \lceil \frac{9k+1}{5} \rceil.$   
\end{proposition}
\begin{IEEEproof}
Let 
$$E'_{adj}=\{\{c_{i},c_{i+1}\}:\{c_{i},c_{i+1}\}\in E_{adj}, \{c_{i},c_{i+1}\}\notin \Earc\}$$ 
be the subset of pairs in $E_{adj}$ that are not in $\Earc$. 
Note that in each round of \textbf{Step 2} in Algorithm~\ref{alg:grouping}, at most $5$ adjacent pairs (corresponding to two choices of $i$ for each $i^*$ and two choices of $j$ for each choice of $i$, plus the pair $\{c_{i^*},c_{i^*+1}\}$) are removed from $E_{adj}$, and thus from $E'_{adj}$ as well. In addition, one pair of nodes in $E'_{adj}$ is added to $E_{group}$ in each round. Since at the \textbf{Initialization} round we have $|E'_{adj}|\ge 2k-1-k=k-1$, there are at least $\frac{k-1}{5}$ rounds. Hence, $E_{group}$ contains at least $\frac{k-1}{5}$ pairs of nodes, and thus $|E_{group}|\le 2k-\frac{k-1}{5}=\frac{9k+1}{5}$. The claimed result follows by observing that the bound has to be integer-valued.  
\end{IEEEproof} 
After obtaining the grouping $E_{group}$, we compute the values of $r_1,\ldots,r_{|E_{group}|}$ in a similar manner to~\eqref{eq:defri1} and~\eqref{eq:defri2}. For $i\in \{1,\ldots, |E_{group}|\}$, let $j_i$ be the $i$th smallest integer $j$ such that $\{c_{j},c_{j+1}\}\in E_{group}$ or $\{c_j\}\in E_{group}$. Let $C=\{(c_j,c_\ell):\exists\, \ell\in \{2,\ldots,2k\} \text{ s.t. } \
\{c_{\ell-1},c_\ell\}\in E_{group},\, \{c_j,c_\ell\}\in \Earc\}.$
Note that for any $j\in \{1,\ldots,2k\}$, there is at most one $\ell\in\{1,\ldots,2k\}$ such that $(c_j,c_\ell)\in C$.
For $i\in \{1,\ldots,|E_{group}|\}$, let 
%\begin{align}\label{eq:defrigeneralk}
%r_i=c_i,\text{ if }c_i\in\
%\end{align}
%and 
\begin{align}\label{eq:defrigeneralk}
&r_i=\nonumber\\
&\begin{cases}c_{j_i},~&\text{if }(c_{j_i},c_\ell)\notin C \text{ for any $\ell\in\{1,\ldots,2k\}$}\\
c_{j_i}-(c_{\ell}-c_{\ell-1}),~& \text{if } i\equiv i^*\bmod 2\text{ and }(c_{j_i},c_\ell)\in C\\
    c_{j_i}+(c_{\ell}-c_{\ell-1}),~& \text{if } i\not\equiv i^*\bmod 2\text{ and }(c_{j_i},c_\ell)\in C
    \end{cases}.
\end{align}
The values of $r_i$, $i\in\{1,\ldots,|E_{group}|\},$ are based on~\eqref{eq:decidingr}. Next, we show that the  $r_i$s, $i\in \{1,\ldots,|E_{group}|\},$ are consistent with the grouping $E_{group}$. First,
\begin{align}\label{eq:groupingk}
c_{j_{i+1}-1}<d_{i}\le c_{j_{i+1}}     
\end{align}
Similar to the proof of Proposition~\ref{prop:k3}, we start by showing that either at least one of 
$r_i=c_{j_i}$ and $r_{i+1}=c_{j_{i+1}}$ holds, or that $\{c_{j_i},c_{j_{i+1}}\}\in \Earc$. If $r_i\ne c_{j_i}$ and $r_{i+1}\ne c_{j_{i+1}}$, then either there exist a $\{i_1,i_1+1\}\in E_{group}$ and a $\{i_2,i_2+1\}\in E_{group}$ such that $\{i_1+1,j_i\}\in \Earc$ (or $i_1+1=j_i$) and $\{i_2+1,j_{i+1}\}\in \Earc$, or $\{c_{j_i-1},c_{j_i}\}\in E_{group}$ $\{c_{j_i},c_{j_{i+1}}\}\in \Earc$. The former case contradicts the \textbf{Step 2} in Algorithm~\ref{alg:grouping} where at least one of the sets $\{i_1,i_1+1\}$ and $\{i_2,i_2+1\}$ is removed from $E_{adj}$ and is not in $E_{group}$. In the latter case, we have that $$d_i= \frac{r_i+r_{i+1}}{2}=\frac{c_{j_{i+1}-1}+c_{j_{i+1}}}{2}\in (c_{j_{i+1}-1},c_{j_{i+1}}).$$
On the other hand, if one of the two equalities $r_i=c_{j_i}$ and $r_{i+1}=c_{j_{i+1}}$ holds, we have that
\begin{align*}
    d_i=\frac{r_i+r_{i+1}}{2}=\frac{c_{j_{i}}+c_{j_{i+1}}\pm (c_{\ell}-c_{\ell-1})}{2}
\end{align*}
for some $(c_{j_i},c_\ell)\in C$ or $(c_{j_{i+1}},c_\ell)\in C$, which implies that $\{c_{\ell-1},c_{\ell}\}\in E_{group}$. Then, since $|c_{\ell-1}-c_{\ell}|$ is the minimum among all pairs in $E_{adj}$ we have that 
$$d_i=\frac{c_{j_{i}}+c_{j_{i+1}}\pm (c_{\ell}-c_{\ell-1})}{2}\in 
(c_{j_{i+1}-1},c_{j_{i+1}}).$$
Otherwise, $\{c_{\ell-1},c_{\ell}\}$ should have been removed in the previous rounds. Finally, if $r_i=c_{j_i}$ and $r_{i+1}=c_{j_{i+1}}$ both hold, we have~\eqref{eq:groupingk}. Thus, we conclude that \eqref{eq:groupingk} holds. The rest of the proof is similar to that of Proposition~\ref{prop:k3}.
